# Supplementary material for: Valid Explanations for Learning to Rank Models
Source: arXiv:2004.13972 source file (2020-05-17)
Supplement: Supplementary file 1 [file appendix_extra.tex]

\begin{table}[]
\label{tab:mslrfull}
\begin{tabular}{lccccccc}
\toprule
% & \multicolumn{7}{c}{k=5} \\
% \midrule
 & \multicolumn{3}{c}{Validity} &  & \multicolumn{3}{c}{Completeness} \\
 & \texttt{Point} & \texttt{Pair} & \texttt{List} &  & \texttt{Point} & \texttt{Pair} & \texttt{List} \\ \midrule
random & 0.002 & 0.009 & 0.000 &  & -0.172 & -0.634 & -0.303 \\
shap1 & 0.006 & 0.050 & 0.023 &  & -0.007 & -0.071 & -0.052 \\
shap5 & 0.009 & 0.048 & 0.001 &  & 0.000 & -0.067 & -0.051 \\ \midrule
\greedy & 0.007 & 0.060 & 0.045 &  & \bf{0.001} & \bf{-0.057} & \bf{-0.034} \\
\greedycov & 0.071 & 0.094 & 0.081 &  & -0.025 & -0.130 & -0.070 \\
\greedycovep & \bf{0.059} & \bf{0.110} & \bf{0.074} &  & 0.020 & -0.074 & -0.041 \\
%\midrule
% c. \greedy & 0.012 & 0.052 & 0.039 &  & 0.002 & -0.056 & -0.019* \\
% c. \greedycov & 0.024 & 0.062 & 0.027 &  & 0.000 & -0.053 & -0.020 \\
% c. \greedycovep & 0.022 & 0.064 & 0.025 &  & -0.013 & -0.061 & -0.014 \\ \midrule

% &  &  &  &  &  &  &  \\

% & \multicolumn{7}{c}{k=10} \\ \midrule
%random & 0.012 & 0.010 & 0.010 &  & -0.109 & -0.479 & -0.175 \\
%shap1 & 0.007 & 0.057 & 0.023 &  & -0.007 & -0.041 & -0.034 \\
%shap5 & 0.010 & 0.083 & 0.031 &  & 0.000 & -0.041 & -0.031 \\ \midrule
%\greedy & 0.011 & 0.098 & 0.058 &  & 0.000 & -0.026 & -0.017 \\
%\greedycov & 0.085 & 0.104 & 0.079 &  & 0.001 & \bf{-0.020} & \bf{-0.015} \\
%\greedycovep & \bf{0.097} & \bf{0.138} & \bf{0.086} &  & -0.002 & -0.055 & -0.031 \\
% \midrule
% c. \greedy & 0.014 &  & 0.035 &  & 0.003 &  & 0.001 \\
% c. \greedycov & 0.013 & 0.091 & 0.033 &  & 0.004 & -0.023 & -0.016 \\
% c. \greedycovep & 0.074 & 0.106 & 0.026 &  & -0.003 & -0.029 & -0.011 \\
\toprule
\end{tabular}
\caption{Results for \textsc{MSLR} when k=5. All greedy approaches are statistically significantly better than the baselines for validity measures. \greedycovep is significantly better than its nearest competitor for validity.}
\end{table}

\begin{table*}[]
\label{tab:mslrfull}
\begin{tabular}{lccccccccccccccc}
\toprule
                             & \multicolumn{7}{c}{k=5}                              &  & \multicolumn{7}{c}{k=10}                     \\
\midrule
 & \multicolumn{3}{c}{Validity} &  & \multicolumn{3}{c}{Completeness} &  & \multicolumn{3}{c}{Validity} &  & \multicolumn{3}{c}{Completeness} \\
                             & point & pair  & list  &  & point  & pair   & list    &  & point & pair & list &  & point & pair & list \\
\midrule
random   & 0.002 & 0.009 & 0.000 &  & -0.172 & -0.634 & -0.303  &  & 0.012 & 0.010 & 0.010 &  & -0.0933 & --     & -0.175 \\
shap1      & 0.006 & 0.050 & 0.023 &  & -0.007 & -0.071 & -0.052  &  & 0.007 & 0.057 & 0.023 &  & -0.007  & -0.041 & -0.034 \\
shap5   & 0.009 & 0.238 & 0.001 &  & 0.000  & -0.067 & -0.051 &  &       &      &      &  & 0.000   & -0.042 & -0.031 \\
\midrule
v. \greedy   & 0.012 & 0.051 & --    &  & 0.008  & -0.053 & --     &  &       &      &      &  & --      & -0.021 & 0.007  \\
v. \greedycov & 0.036 & --    & --    &  & --     & --     & --     &  &       &      &      &  & 0.007   & -0.021 & --     \\
v. \greedycovep & 0.065 & 0.111 & 0.077 &  & 0.012 & -0.067 & -0.045 &  & 0.078 & 0.037 & 0.029 &  & -0.006 & -0.057 & -0.033 \\
\midrule
c. \greedy & 0.012    & 0.052   & 0.039   &  & 0.002     & -0.056   & -0.019*   &  &          &         &         &  & 0.002     & -0.021    & -0.018   \\
c. \greedycov  & 0.024    & 0.062   & 0.027   &  & 0.000     & -0.053   & -0.020    &  &          &         &         &  & 0.000     & -0.022    & -0.004   \\
c. \greedycovep & 0.022 & 0.064 & 0.025 &  & -0.013 & -0.061 & -0.014 &  & 0.072 & 0.099 & 0.028 &  & -0.005 & -0.028 & -- \\
\toprule
\end{tabular}
\caption{Results for the \textsc{MSLR} when k=5,10. Approaches prefixed with $c$ refer to completeness optimized whereas $v$ refers to validity optimized.}
\end{table*}

\begin{table}[]
\small
\label{tab:mean}
\begin{tabular}{lccccccc}
\toprule
                        & \multicolumn{3}{c}{MQ2008} &  & \multicolumn{3}{c}{MSLR} \\
                        & point   & pair    & list   &  & point   & pair   & list  \\
\midrule
random                  & -0.045  & -0.241  & -0.132 &  &     -0.085    &   0.010     &  -0.142     \\
shap1                   & 0.085   & -0.068  & 0.028  &  &      0.000   &     -0.152   &   -0.015    \\
shap5                   & 0.087   & -0.061  & 0.052  &  &      0.004   &     0.085   &    -0.025   \\
\midrule
v. \greedy            & 0.134   & --      & 0.089  &  &         &        &       \\
v. \greedycov         & 0.120*  & -0.050  & 0.094  &  &         &        &       \\
v. \greedycovep & 0.143   & -0.003  & 0.100  &  &         &        &       \\
\midrule
c. \greedy              & 0.107   & -0.130  & 0.054  &  &         &        &       \\
c. \greedycov         & 0.075   & -0.044  & 0.025  &  &         &        &       \\
c. \greedycovep & 0.113   & -0.098  & 0.037  &  &         &        &      \\
\toprule
\end{tabular}
\caption{Results for the mean of completeness and validity for \textsc{MQ2008, MSLR} when k=5. Approaches prefixed with $c$ refer to completeness optimized whereas $v$ refers to validity optimized.}
\end{table}
