# Supplementary material for: Valid Explanations for Learning to Rank Models
Source: arXiv:2004.13972 source file (2020-05-17)
Supplement: Supplementary file 2 [file appendix.tex]

\appendix
